# Supplementary material for: Effect of the atomic structure of complexions on the active disconnection mode during shear-coupled grain boundary motion
Source: arXiv:2305.10275 ancillary file (2024-05-10)
Supplement: Supplementary file 1 [file Supplemental.pdf]

Supplemental Material

# Effect of the atomic structure of complexions on the active disconnection mode during shear-coupled grain boundary motion

Swetha Pemma,[1] Rebecca Janisch,[2] Gerhard Dehm,[1] and Tobias Brink[1]

[1] *Max-Planck-Institut für Eisenforschung GmbH, Max-Planck-Straße 1, 40237 Düsseldorf, Germany*
[2] *Interdisciplinary Centre of Advanced Materials Simulation (ICAMS), Ruhr-Universität Bochum, 44780 Bochum, Germany*

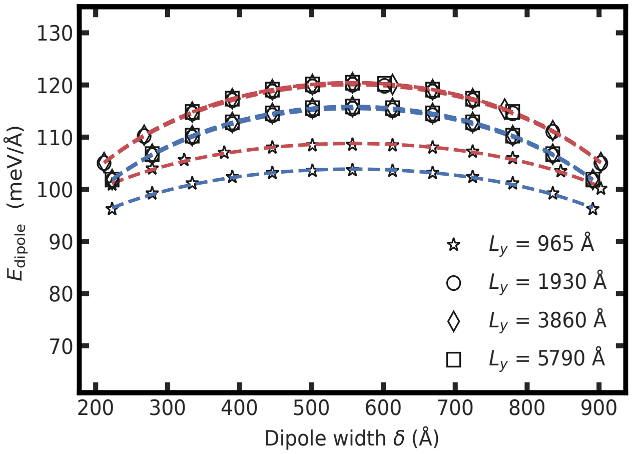


FIG. S1. Convergence of the disconnection dipole energy $E_{\mathrm{dipole}}$ with the system size $L_y$ in the direction normal to the GB. Data for $\Sigma19$b GBs. The energies are plotted for different dipole widths $\delta$. Symbols represent the investigated system sizes, while red lines are GBs with domino complexions and blue lines are GBs with pearl complexions. The dipole energies converge at $L_y \geq 1930$ Å, indicating that the interaction between surfaces and GBs becomes negligible.

TABLE S1. Disconnection dipole parameters obtained from fitting Eq. 5 in the main paper to $E_{\mathrm{dipole}}$ from the simulations of $\Sigma19$b GBs (Fig. S1). In addition to the data in Table II in the main paper, the values for different system sizes $L_y$ in the direction normal to the GB are provided. We list the system size $L_y$, the parameter $K$ describing anisotropic crystal elasticity, the effective disconnection core size $\delta_0$, the dipole energy $E^*_{\mathrm{dipole}}$ for $\delta = L_x/2$, as well as the dipole energy differences $\Delta E^*_{\mathrm{dipole}} = E^{*\,\mathrm{domino}}_{\mathrm{dipole}} - E^{*\,\mathrm{pearl}}_{\mathrm{dipole}}$. As an additional convergence parameter, we also made sure that $\gamma^* = (E_1 - E_{\mathrm{fcc}})/(L_x L_y)$ is converged. This value represents the GB energy of the complexion plus the energy of a disconnection dipole with width $\delta = L_x/2$, where $E_1$ is the energy of a system containing the GB plus dipole, $E_{\mathrm{fcc}}$ is the energy of the same system without a GB.

| $L_y$ (Å) | 964.490 | 1929.540 | 3859.800 | 5790.070 |
|---|---|---|---|---|
| $\gamma^*_{\mathrm{domino}}$ (J/m$^2$) | 0.872 | 0.873 | 0.873 | 0.873 |
| $K_{\mathrm{domino}}$ (meV/Å$^3$) | 41.9 | 75.6 | 77 | 76.8 |
| $\delta_0^{\mathrm{domino}}$ (Å) | 0.191 | 3.540 | 3.791 | 3.761 |
| $\gamma^*_{\mathrm{pearl}}$ (J/m$^2$) | 0.836 | 0.837 | 0.837 | 0.837 |
| $K_{\mathrm{pearl}}$ (meV/Å$^3$) | 40.6 | 75 | 76.4 | 76.4 |
| $\delta_0^{\mathrm{pearl}}$ (Å) | 0.211 | 4.067 | 4.358 | 4.366 |
| $\Delta E^*_{\mathrm{dipole}}$ (meV/Å) | 4.885 | 4.567 | 4.557 | 4.555 |

TABLE S2. The disconnection energies of disconnection monopoles $E_{\mathrm{monopole}}$ (single disconnection on a GB with open boundary conditions in $x$ direction) do not converge, because the strain energy of a disconnection/dislocation scales proportionally to $\ln R/\delta_0$, where $R$ is a measure of the system size (here calculated for two values of $L_x$). However, the difference $\Delta E_{\mathrm{monopole}} = E^{\mathrm{domino}}_{\mathrm{monopole}} - E^{\mathrm{pearl}}_{\mathrm{monopole}}$ is converged. The data comes from simulations for $\Sigma19$b GBs with $L_y = 5790.070$ Å.

| $L_x$ (Å) | 2229.363 | 3342.799 |
|---|---|---|
| $E^{\mathrm{domino}}_{\mathrm{monopole}}$ (meV/Å) | 68.583 | 73.506 |
| $E^{\mathrm{pearl}}_{\mathrm{monopole}}$ (meV/Å) | 65.751 | 70.699 |
| $\Delta E_{\mathrm{monopole}}$ (meV/Å) | 2.832 | 2.807 |

## I. BURGERS CIRCUIT MAPPING

In order to confirm the Burgers vectors and step heights of the constructed disconnection dipoles in all our complexions, we constructed Burgers circuits. In Fig. 4 in the main text, the Burgers circuits (black atoms) start and end at same structural unit. We can thus elide the GB crossings, which are equivalent and thus cancel out each other, and only deal with the circuit in the perfect fcc lattices [1–3]. We arrive at two lattice translation vectors, one in the top and one in the bottom crystal ($\mathbf{t}_1$ and $\mathbf{t}_2$). The translation vectors $\mathbf{t}_1$ and $\mathbf{t}_2$ are then transposed into the dichromatic pattern, by following the sites of the top and bottom grain, respectively (Figs. S2 and S3). The difference between the vectors $\mathbf{t}_1$ and $\mathbf{t}_2$ is the Burgers vector

$$\mathbf{b} = \mathbf{t}_1 - \mathbf{t}_2. \tag{1}$$

The step heights $h_1$ and $h_2$ are the heights from the coincidence site (O) to the ends of the half-circuits $\mathbf{t}_1$ and $\mathbf{t}_2$. Since our disconnections have Burgers vectors that lay within the GB plane, the step height of the disconnection is simply

$$h = h_1 = h_2. \tag{2}$$


[1] R. Pond, TEM studies of line defects in interfaces, Ultramicroscopy **30**, 1 (1989).

[2] A. Rajabzadeh, F. Mompiou, S. Lartigue-Korinek, N. Combe, M. Legros, and D. Molodov, The role of disconnections in deformation-coupled grain boundary migration, Acta Materialia **77**, 223 (2014).

[3] D. L. Medlin, K. Hattar, J. A. Zimmerman, F. Abdeljawad, and S. M. Foiles, Defect character at grain boundary facet junctions: Analysis of an asymmetric $\Sigma = 5$ grain boundary in Fe, Acta Mater. **124**, 383 (2017).

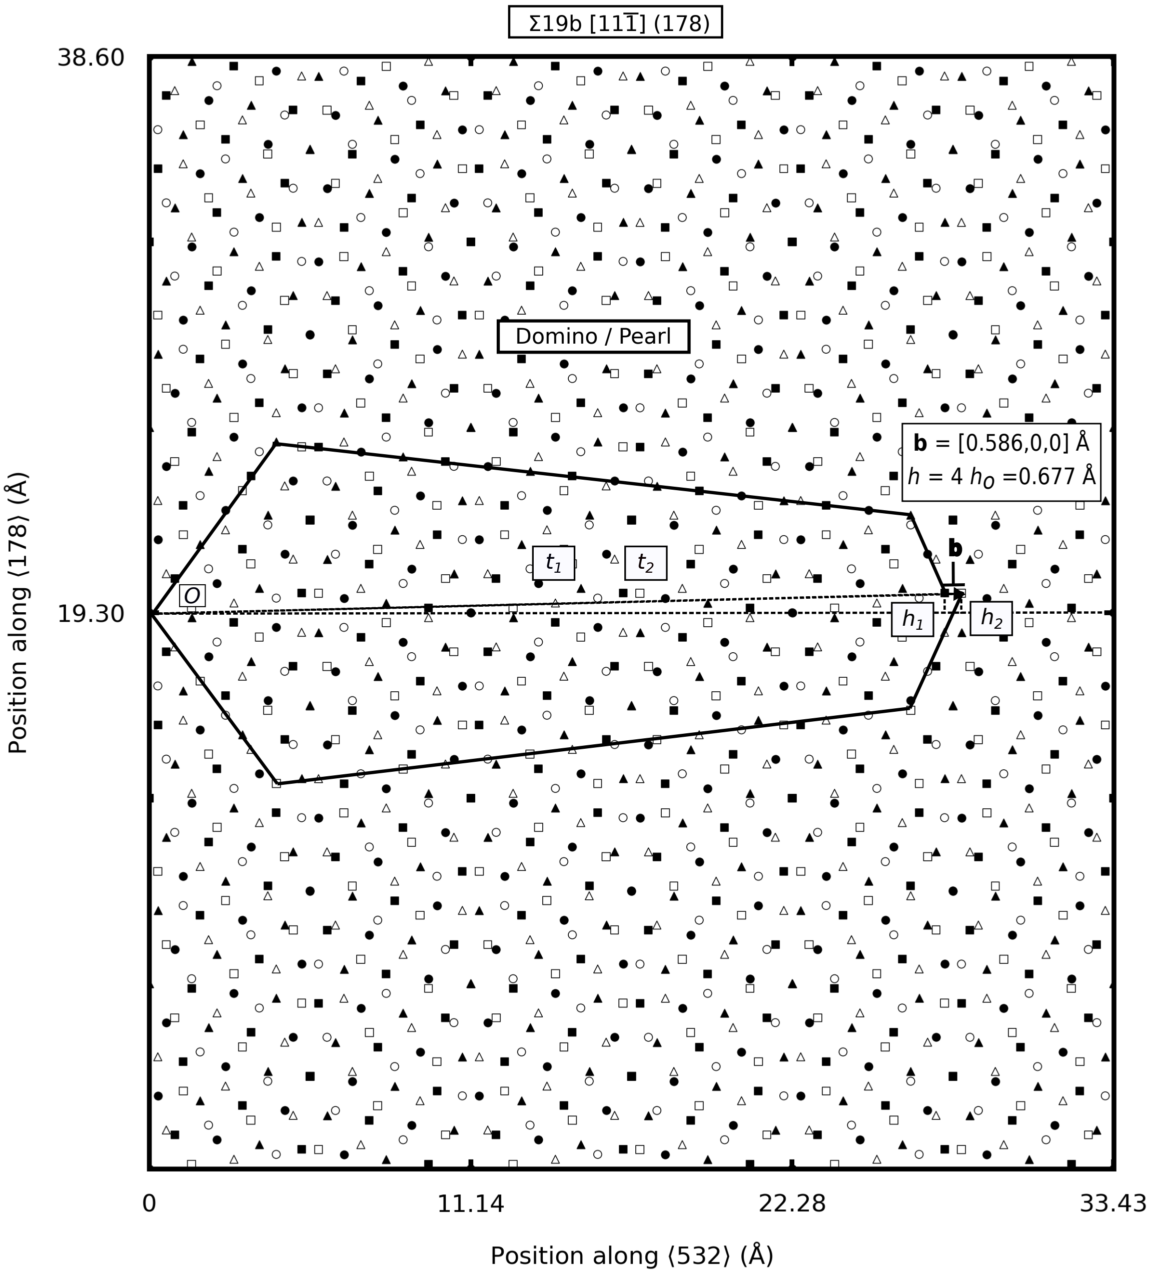


FIG. S2. The Burgers vector **b** and step height $h$ of the disconnection present at Σ19b GBs during shear-coupled motion can be obtained by Burgers circuit mapping in the dichromatic pattern (see also supplemental text above). The vectors $\mathbf{t}_1$ and $\mathbf{t}_2$ are transposed from the Burgers circuits in Fig. 4(a)–(b) of the main text into the dichromatic pattern. The difference in vectors $\mathbf{t}_1$ and $\mathbf{t}_2$ starting from the same coincidence site O is the Burgers vector. The vertical lines from the end of $\mathbf{t}_1$ and $\mathbf{t}_2$ dropped to the horizontal line which passes through the coincidence site O correspond to the step heights $h_1$ and $h_2$. Since **b** is horizontal (conservative shear-coupling mode), it is $h_1 = h_2$.

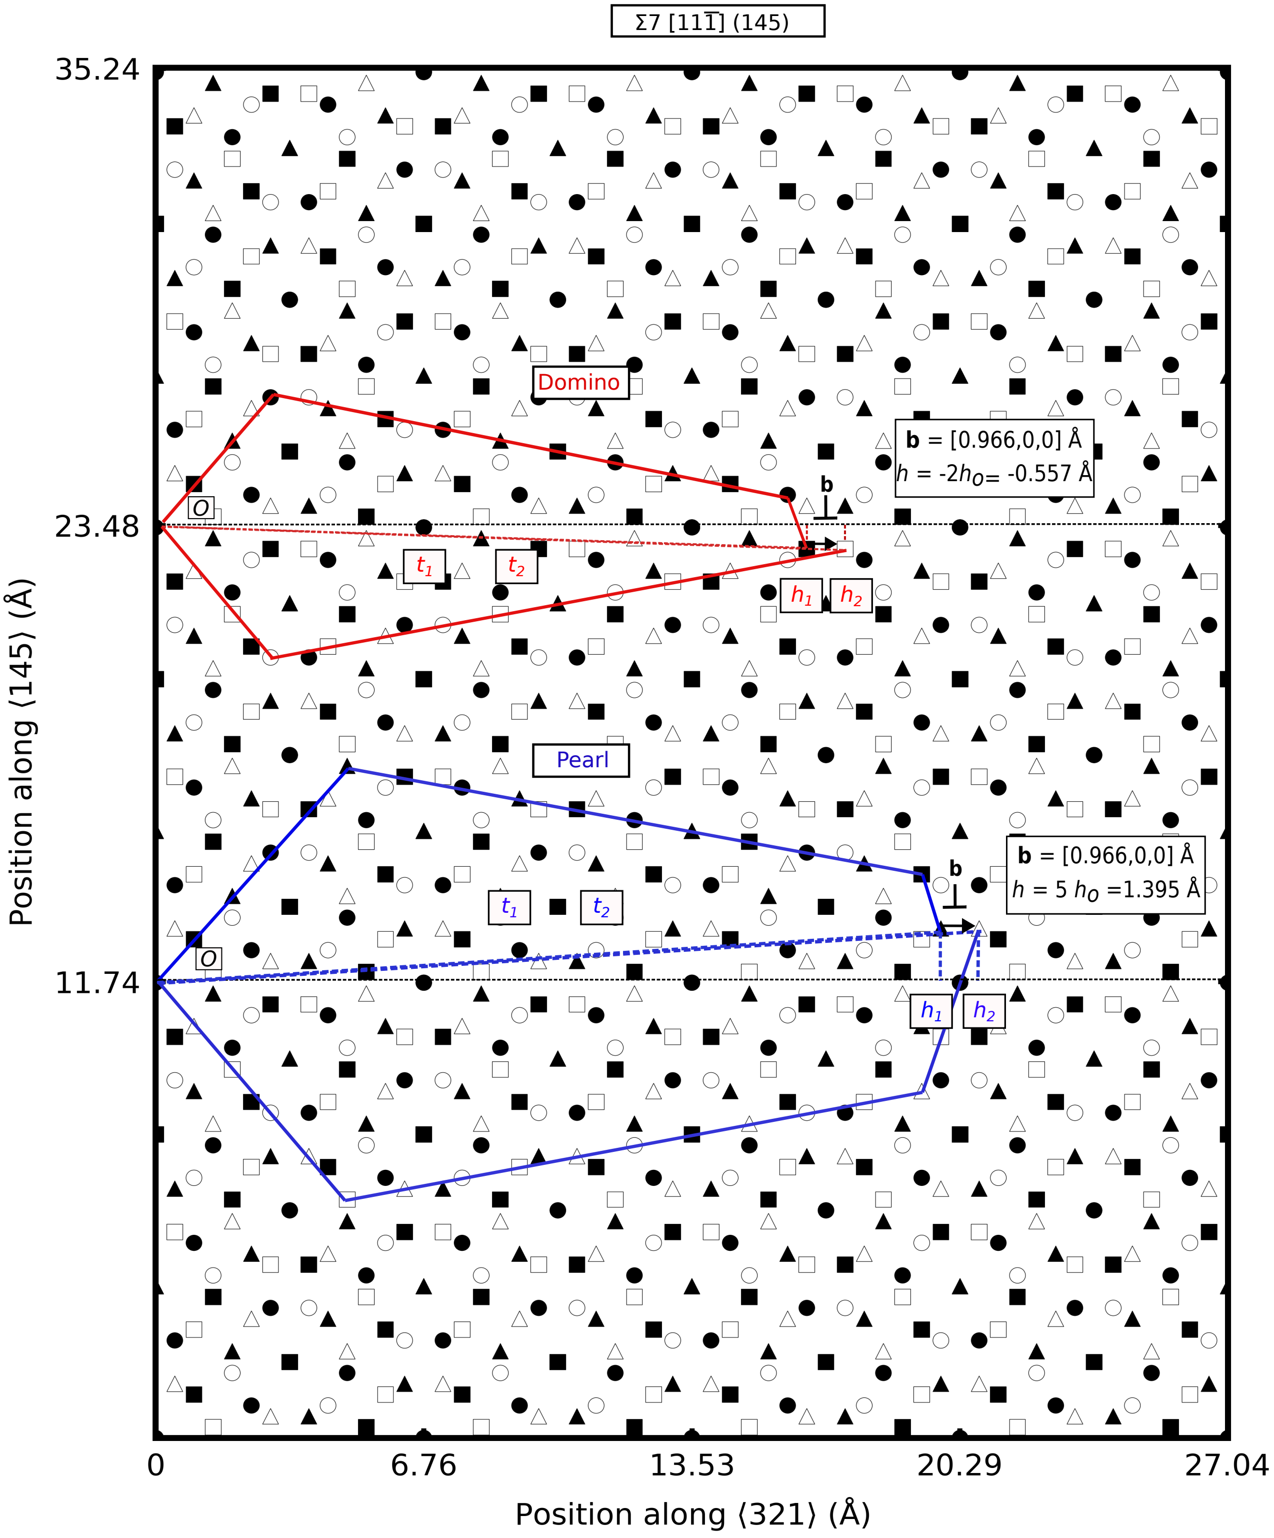


FIG. S3. The Burgers vector **b** and step height $h$ of the disconnections present at Σ7 GBs, which differ for pearl and domino complexions (cf. Fig. S2 for the method). The vectors $\mathbf{t}_1$ and $\mathbf{t}_2$ are transposed from the Burgers circuits in Fig. 4(c)–(d) of the main text into the dichromatic pattern. Here, this is repeated separately for pearl and domino, which differ in step height. The difference in vectors $\mathbf{t}_1$ and $\mathbf{t}_2$ starting from the same coincidence site O is the Burgers vector. The vertical lines from the end of $\mathbf{t}_1$ and $\mathbf{t}_2$ dropped to the horizontal line which passes through the coincidence site O correspond to the step heights $h_1$ and $h_2$. Since **b** is horizontal (conservative shear-coupling mode), it is $h_1 = h_2$.

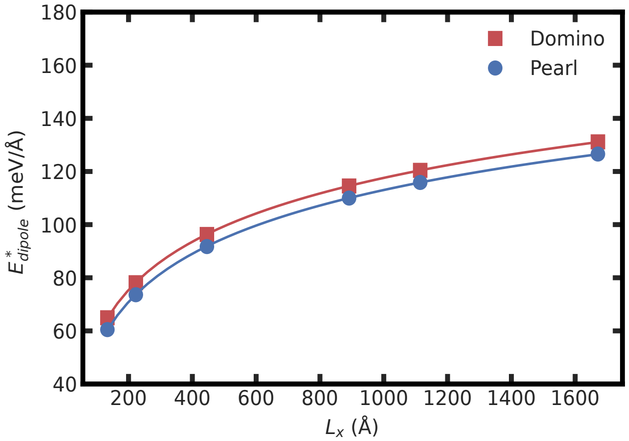


FIG. S4. Dependence of the disconnection dipole energy $E^*_{\mathrm{dipole}}$ for $\delta = L_x/2$ on the system size $L_x$. The data follows the expected trend according to Eq. 6 in the main paper. The difference between domino and pearl complexions is constant, as expected.

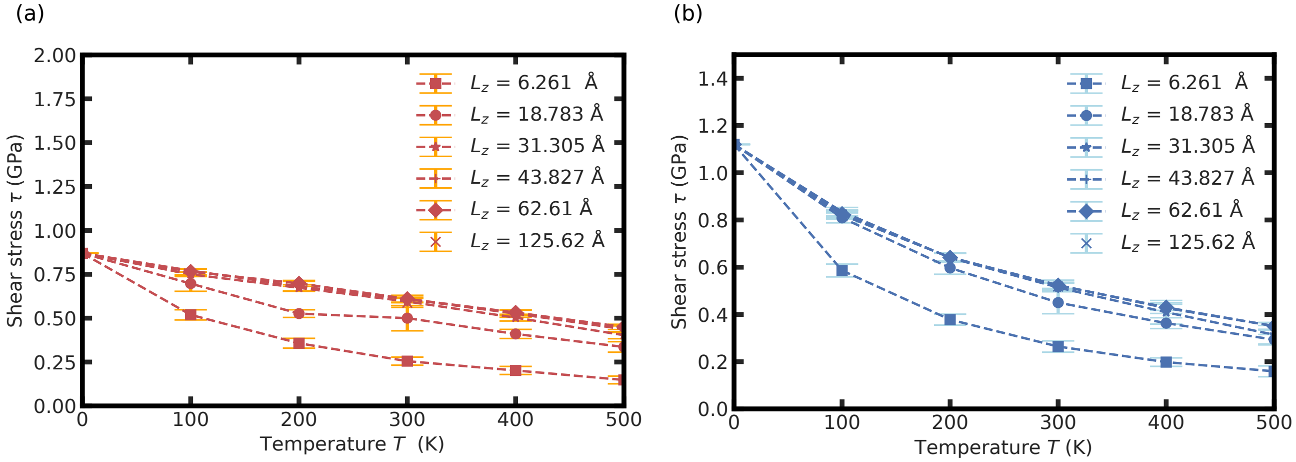


FIG. S5. The critical shear stress in Σ19b GBs with (a) domino and (b) pearl complexions was calculated for different $L_z$ and for different temperatures. The values start to converge at $L_z \geq 31.305$ Å. This shows that the 2D model, which predicts constant critical shear stress independent of $L_z$ applies to our thin systems.

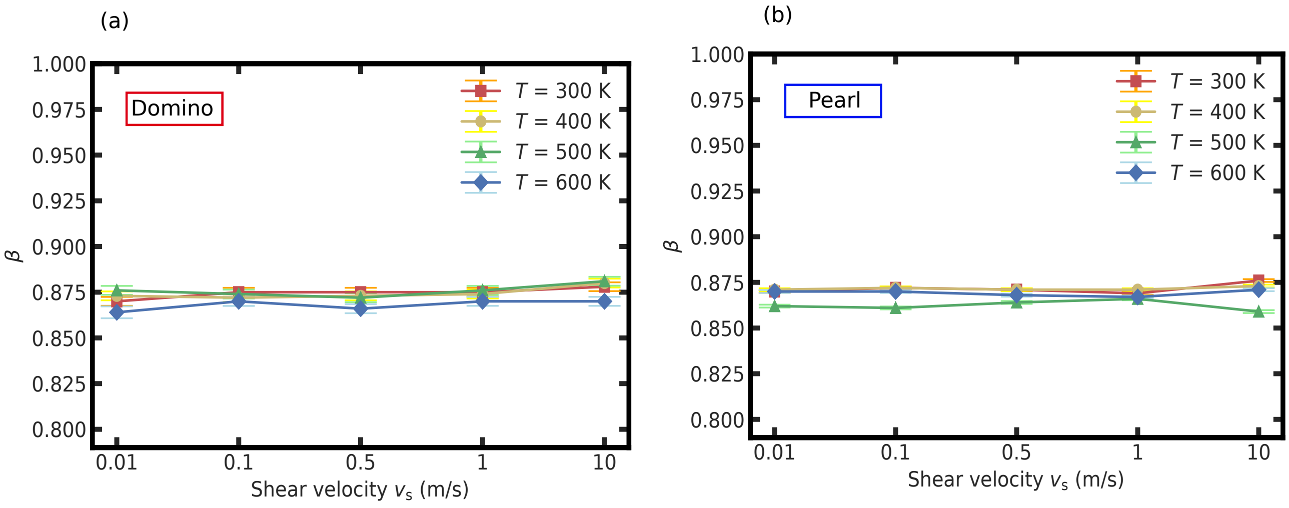


FIG. S6. The shear coupling factor of (a) domino and (b) pearl complexions in Σ19b GBs was calculated for different shear velocities at four different temperatures. It did not vary for the investigated shear velocities and temperatures.
